# Supplementary material for: PSD: Pushing the Pareto Frontier of Diffusion LLMs via Parallel Speculative Decoding
Source: arXiv:2605.15609 source file (2026-05-15)
Supplement: Supplementary file 1 [file 08_appendix.tex]

% \clearpage
% \appendix
% \renewcommand{\thesection}{\Alph{section}}
% \section{Appendix}\label{sec:appendix}
